# Supplementary material for: Multi-Head Graph Convolutional Network for Structural Connectome Classification
Source: arXiv:2305.02199 source file (2023-09-20)
Supplement: Supplementary file 1 [file supplementary.tex]

\begin{table}
\caption{Classification results using comparative (graph) DL methods}\label{tab1}
\begin{tabular}{|l|l|l|}
\hline
Dataset/Model Type &OASIS3 &PreventAD \\
\hline
MLP &85.77 \pm 6.80 &86.15 \pm 13.10\\
DGCNN & 76.37 \pm 3.80 & 80.02 \pm 4.80  \\
GCNConv &83.00 \pm 4.04 &86.81 \pm 5.80\\
Graphconv  & 75.70 \pm 3.30 & 80.32 \pm 6.21\\
ResGatedGraphConv & 77.69 \pm 3.05 & 81.08 \pm 6.40\\
GINConv & 75.50 \pm 4.2 &82.66 \pm 3.03\\
GCNconv,emb size 50 Skipcon, aug & 83.60 \pm 6.50 &87.50 \pm 5.60\\
%3head,GCNconv,GCNconv,Linear,flattening &87.84 \pm 6.60 & 89.50 \pm 6.10\\
%3head,GCNconv,GCNconv,Linear,flattening, aug & 88.53 \pm 4.12 & 90.60 \pm 6.80\\
\hline
\end{tabular}
\end{table}

\begin{table}
\caption{Dataset partition}\label{tab1}
\begin{tabular}{|l|l|l|l|l|l|}
\hline
Name&Total size&Size-10\% &Male &Female&Ratio\\
PREVENT--AD& 789 &710 &199 &511 &0.73 \\
OASIS3 &1294 &1164 &515 &649 &0.56 \\
\hline
\end{tabular}
\end{table}
